# Supplementary material for: Minimum measurements quantum protocol for band structure calculation
Source: arXiv:2511.04389 ancillary file (2026-06-15)
Supplement: Supplementary file 1 [file Supplementary_Information_final.pdf]

# Supplementary Information for “Minimum Measurements Quantum Protocol for Band Structure Calculations”

Michal Krejčí<sup>1,2</sup>, Lucie Krejčí<sup>1</sup>, Ijaz Ahamed Mohammad<sup>3</sup>, Martin Plesch<sup>3,4</sup>, Martin Friák<sup>1,2\*</sup>

<sup>1</sup>Institute of Physics of Materials, v. v. i., Czech Academy of Sciences, Žitkova 22, Brno, 616 00 Czech Republic.

<sup>2</sup>Department of Condensed Matter Physics, Faculty of Science, Masaryk University, Kotlářská 2, Brno, 611 37, Czech Republic.

<sup>3</sup>Institute of Physics, Slovak Academy of Sciences, Dúbravská cesta 9, Bratislava 45, 845 11, Slovak Republic.

<sup>4</sup>Faculty of Natural Sciences, Matej Bel University, Tajovského 40, Banská Bystrica, 974 09, Slovak Republic.

## Supplementary Note 1 – Derivation of the Qubit Hamiltonian

Exploiting the hermiticity  $\mathcal{H}^\dagger = \mathcal{H}$  of the tight-binding Hamiltonian, Eq. (1) in the main text, we can rewrite it in the more convenient form

$$\hat{\mathcal{H}}(\mathbf{k}) = \sum_j \varepsilon_j \hat{c}_{\mathbf{k}j}^\dagger \hat{c}_{\mathbf{k}j} + 2 \sum_j \sum_{l>j} \text{Re} \left\{ \mathcal{H}_{jl}(\mathbf{k}) \hat{c}_{\mathbf{k}j}^\dagger \hat{c}_{\mathbf{k}l} \right\}. \quad (1)$$

Using the mapping, see Eq. (3) in the main text, between the creation and annihilation operators and the Pauli operators, we can rewrite the first term in the Hamiltonian (1) as

$$\hat{c}_{\mathbf{k}j}^\dagger \hat{c}_{\mathbf{k}j} = \frac{1}{4} \left( \hat{X}_j - i\hat{Y}_j \right) \left( \hat{X}_j + i\hat{Y}_j \right) = \frac{1}{4} \left( \hat{X}_j^2 + \hat{Y}_j^2 + i\hat{X}_j\hat{Y}_j - i\hat{Y}_j\hat{X}_j \right) = \frac{1}{2} \left( \hat{I} - \hat{Z}_j \right). \quad (2)$$

For the second term in the Hamiltonian (1), we get

$$\hat{c}_{\mathbf{k}j}^\dagger \hat{c}_{\mathbf{k}l} = \frac{1}{4} \left( \hat{X}_j - i\hat{Y}_j \right) \left( \hat{X}_l + i\hat{Y}_l \right) = \frac{1}{4} \left( \hat{X}_j\hat{X}_l + \hat{Y}_j\hat{Y}_l \right) + \frac{i}{4} \left( \hat{X}_j\hat{Y}_l - \hat{Y}_j\hat{X}_l \right) \quad (3)$$

and taking the real part of the expression  $2\text{Re} \left\{ \mathcal{H}_{jl} \hat{c}_{\mathbf{k}j}^\dagger \hat{c}_{\mathbf{k}l} \right\}$  gives us

$$\begin{aligned} 2\text{Re} \left\{ \mathcal{H}_{jl} \hat{c}_{\mathbf{k}j}^\dagger \hat{c}_{\mathbf{k}l} \right\} &= \left[ \frac{\mathcal{H}_{jl}}{4} \left( \hat{X}_j\hat{X}_l + \hat{Y}_j\hat{Y}_l \right) + \frac{i\mathcal{H}_{jl}}{4} \left( \hat{X}_j\hat{Y}_l - \hat{Y}_j\hat{X}_l \right) \right] \\ &\quad + \left[ \frac{\mathcal{H}_{jl}^*}{4} \left( \hat{X}_j\hat{X}_l + \hat{Y}_j\hat{Y}_l \right)^\dagger - \frac{i\mathcal{H}_{jl}^*}{4} \left( \hat{X}_j\hat{Y}_l - \hat{Y}_j\hat{X}_l \right)^\dagger \right] \\ &= \frac{1}{2} \text{Re} \{ \mathcal{H}_{jl} \} \left( \hat{X}_j\hat{X}_l + \hat{Y}_j\hat{Y}_l \right) + \frac{1}{2} \text{Im} \{ \mathcal{H}_{jl} \} \left( \hat{Y}_j\hat{X}_l - \hat{X}_j\hat{Y}_l \right), \end{aligned} \quad (4)$$

where we have used the fact that  $\left( \hat{X}_j\hat{X}_l \right)^\dagger = \hat{X}_j\hat{X}_l$ , and  $\left( \hat{Y}_j\hat{Y}_l \right)^\dagger = \hat{Y}_j\hat{Y}_l$  because  $\hat{X}$ , and  $\hat{Y}$  are hermitian. Similarly for  $\hat{Y}_j\hat{Y}_l$ ,  $\hat{X}_j\hat{Y}_l$ , and  $\hat{Y}_j\hat{X}_l$  terms. The qubit Hamiltonian is therefore

$$\hat{\mathcal{H}}(\mathbf{k}) = \frac{1}{2} \sum_j \varepsilon_j (\hat{I} - \hat{Z}_j) + \frac{1}{2} \sum_j \sum_{l>j} \text{Re} \{ \mathcal{H}_{jl}(\mathbf{k}) \} \left( \hat{X}_j\hat{X}_l + \hat{Y}_j\hat{Y}_l \right) + \frac{1}{2} \sum_j \sum_{l>j} \text{Im} \{ \mathcal{H}_{jl}(\mathbf{k}) \} \left( \hat{Y}_j\hat{X}_l - \hat{X}_j\hat{Y}_l \right). \quad (5)$$

The first term in the Hamiltonian (5) represents the on-site energies, and the second and third terms together represent the hopping processes between orbitals  $j$  and  $l$ .

## Supplementary Note 2 – Variational Quantum Deflation

An example of a quantum algorithm capable of obtaining the band structure even on current (Noisy-Intermediate-Scale-Quantum) NISQ devices [1] is the Variational Quantum Deflation (VQD) algorithm [2], an extension of the Variational Quantum Eigensolver (VQE) [3]. Unlike VQE, which computes only the energy eigenvalue of the ground state, VQD can also calculate excited states.

To obtain the band structure, one must first evaluate the expectation value of the qubit Hamiltonian with respect to a trial state. That is, evaluate the expectation values of the corresponding Pauli operators appearing in Eq. (5). A typical VQD subroutine for calculating excited-state eigenvalues modifies the original Hamiltonian by adding a penalty term. The so-called VQD cost function for the  $n$ -th excited state is given by

$$\langle \psi(\boldsymbol{\theta}) | \hat{\mathcal{H}}_n(\mathbf{k}) | \psi(\boldsymbol{\theta}) \rangle = \langle \psi(\boldsymbol{\theta}) | \hat{\mathcal{H}}(\mathbf{k}) | \psi(\boldsymbol{\theta}) \rangle + \sum_{i=0}^{n-1} \beta_i |\langle \psi(\boldsymbol{\theta}) | \psi(\boldsymbol{\theta}^i) \rangle|^2. \quad (6)$$

The classical optimizer then minimizes this cost function to obtain the parameters of the quantum circuit  $\boldsymbol{\theta}^n$  that define the eigenstate

$$\min_{\boldsymbol{\theta}} \langle \psi(\boldsymbol{\theta}) | \hat{\mathcal{H}}_n(\mathbf{k}) | \psi(\boldsymbol{\theta}) \rangle \rightarrow \boldsymbol{\theta}^n, \quad (7)$$

where  $\boldsymbol{\theta}^n$  are the values of the variational parameters for which the cost function (6) is minimized. The energy eigenvalues are then calculated as the expectation value of the original unmodified Hamiltonian with respect to the eigenstate  $|\psi(\boldsymbol{\theta}^n)\rangle$

$$E_n(\mathbf{k}) = \langle \psi(\boldsymbol{\theta}^n) | \hat{\mathcal{H}}(\mathbf{k}) | \psi(\boldsymbol{\theta}^n) \rangle. \quad (8)$$

For  $n = 0$ , this is the ground state, and the VQD cost function is only the first term in Eq. (6). This is identical to the VQE cost function. For excited states  $n = 1, 2, \dots, N - 1$ , additional penalty terms must be added to ensure orthogonality between the previously found states. This corresponds to the second term in (6). The VQD calculates eigenstates iteratively; to obtain the  $n$ -th excited state, one must first know the previously found parameters  $\boldsymbol{\theta}^0, \boldsymbol{\theta}^1 \dots \boldsymbol{\theta}^{n-1}$  and eigenstates  $|\psi(\boldsymbol{\theta}^0)\rangle, |\psi(\boldsymbol{\theta}^1)\rangle, \dots, |\psi(\boldsymbol{\theta}^{n-1})\rangle$ . This procedure is performed iteratively for each  $\mathbf{k}$ -point.

In addition, one must specify the parameters  $\beta_i$  appearing in Eq. (6). For the  $n$ -th excited state, the parameters must satisfy the inequality  $\beta_i > E_n(\mathbf{k}) - E_i(\mathbf{k})$ , to ensure orthogonality between the previously found eigenstates, as shown in [2]. However, there is a subtle issue: the eigenenergies  $E_n(\mathbf{k})$  are not known a priori; they are precisely what VQD aims to calculate at this step. To ensure that the above inequality is always satisfied for each  $\mathbf{k}$  point, we choose  $\beta_i = 2\Delta$  where  $\Delta = \sum_j \varepsilon_j + \sum_{j,l>j} |(\mathcal{H}_{jl}(\mathbf{k}))|$ . Lastly, to calculate the overlap term appearing in the modified cost function (6), we implemented the so-called low-depth method [2, 4] by using the inverse of the quantum circuit for the variational ansatz. The implementation of VQD involves three key subroutines.

- *State preparation:* As in any variational method in quantum mechanics, we must propose a trial wavefunction  $|\psi(\boldsymbol{\theta})\rangle$ , which depends on a set of variational parameters  $\boldsymbol{\theta}$ . This trial state is constructed with a quantum computer and is represented as a parameterized quantum circuit.
- *Expectation value estimation:* The second step involves estimating the VQD cost function defined in Eq. (6). For each  $\mathbf{k}$  point and eigenstate, the VQD algorithm evaluates this cost function on a quantum computer to obtain an estimate of the corresponding energy. In the main text, we proposed an efficient measurement strategy for this evaluation, which requires only three Pauli measurement settings, independent of system size, compared to the conventional  $\mathcal{O}(N)$  measurement rounds.
- *Classical optimization:* The third step is classical optimization, in which the variational parameters  $\boldsymbol{\theta}$  are updated to minimize the energy. In the main text, we used a local optimization method combined with a bootstrapping, or “warm-start,” strategy, which is a heuristic method for selecting initial variational parameters when solving a sequence of related problems. In our case, computing the band structure across different  $\mathbf{k}$  points along the high symmetry path in the first Brillouin zone. The cost function estimation on quantum hardware is currently expensive, making the use of local optimization particularly important in variational algorithms, as it incurs significantly less computational overhead than global methods.

## Supplementary Note 3 – State preparation

Given the reciprocal orbital qubit mapping, see Eq. (3) in the main text, used to transform the creation and annihilation operators into qubit operators, the most straightforward and intuitive trial state can be constructed as follows. Since the TB model is a single-electron model, one can consider only the subspace of Hilbert space that is spanned by the following  $N$ -qubit basis states

$$|e_j\rangle = \hat{c}_{\mathbf{k}j}^\dagger |0\rangle, \quad j = 0, 1, \dots, N - 1, \quad (9)$$

where  $|0\rangle$  represents "vacuum" of empty orbitals. In the computational basis, these are precisely the states with a Hamming weight of 1, meaning exactly one qubit is in the  $|1\rangle$  (occupied) state while the rest are  $|0\rangle$  (empty) states. There are exactly  $N$  such states for  $N$ -qubit model. A natural choice for the initial trial state is therefore a superposition of all basis states with Hamming weight 1, that is

$$|\psi(\boldsymbol{\theta})\rangle = \sum_{j=0}^{N-1} a_j |e_j\rangle, \quad (10)$$

where the coefficients of the linear combination  $a_j$  depend on the variational parameters  $\boldsymbol{\theta}$ .

An efficient method for preparing the state (10) on a quantum computer was introduced in Ref. [5], first demonstrated for the tight-binding Hamiltonian by Sherbert *et al.* [6, 7], and has been further validated in our recent works [8, 9]. The key component of this method is a two-qubit entangling gate, denoted here as the A-gate which can be decomposed into three two-qubit control operations, CNOTs, two parameterized one-qubit rotations  $R_Z$ , and two parameterized one-qubit rotations  $R_Y$ , see Fig. 1.

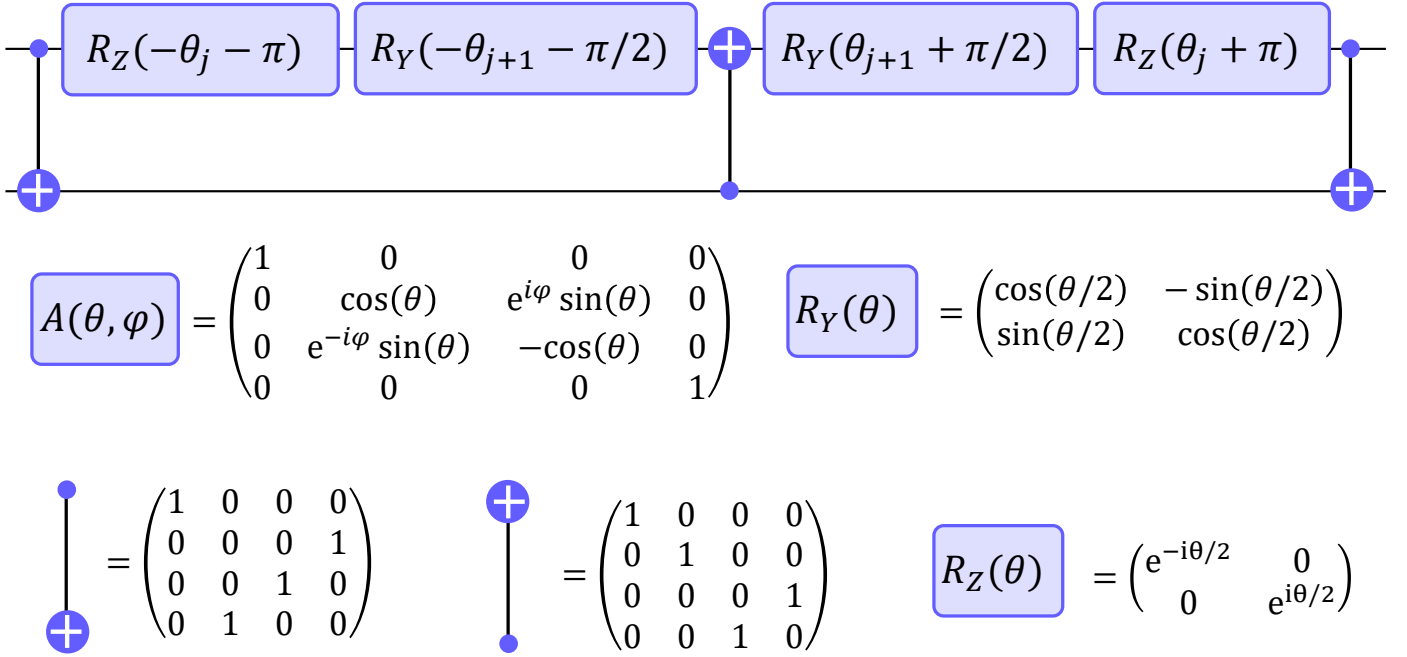

**Fig. 1:** Decomposition of two-qubit A-gate into two-qubit controlled operations and four one-qubit rotations, in particular two  $R_Y$  and two  $R_Z$ .

The trial state (10), which is a superposition of basis states with Hamming weight 1, is then constructed by successive application of A-gates on the initial state  $\hat{X}_0 |0\rangle$ , applied to all neighbouring qubits, and is given by the following formula

$$|\psi(\boldsymbol{\theta})\rangle = \prod_{j=0}^{N-2} \hat{A}_{j+1,j} \hat{X}_0 |0\rangle. \quad (11)$$

The initial state  $\hat{X}_0 |0\rangle$  just creates a single-electron occupation state, and the successive application of  $\hat{A}_{j+1,j}$  gates on neighboring qubits in the quantum register generates a superposition of states with Hamming weight 1, see Fig. 2. Each  $\hat{A}_{j+1,j}$  gate depends on two angles  $\theta_{j+1}, \theta_j$ , and for an  $N$ -qubit model, a total of  $N - 1$  A-gates are needed to span the entire subspace of Hilbert space with the Hamming weight of 1. Therefore, the variational ansatz generally depends on  $2(N - 1)$  variational parameters. Optionally, one could apply an extra layer of A-gates to construct a more expressive trial state as was done in our previous work [9]. While this increased expressivity may lead to more accurate energy estimations, it comes at the cost of added quantum gate overhead, e.g., an additional source of noise in quantum hardware, and a more complex optimization landscape due to additional variational parameters.

## Supplementary Note 4 – Cost Function for Tight-binding Hamiltonians

In the following, we analyze the expectation values of the Pauli operators appearing in the qubit Hamiltonian (5) with respect to the trial state (10) and construct the resulting cost function as  $E(\mathbf{k}, \boldsymbol{\theta}) = \langle \hat{\mathcal{H}} \rangle$ . In general, the trial state is the

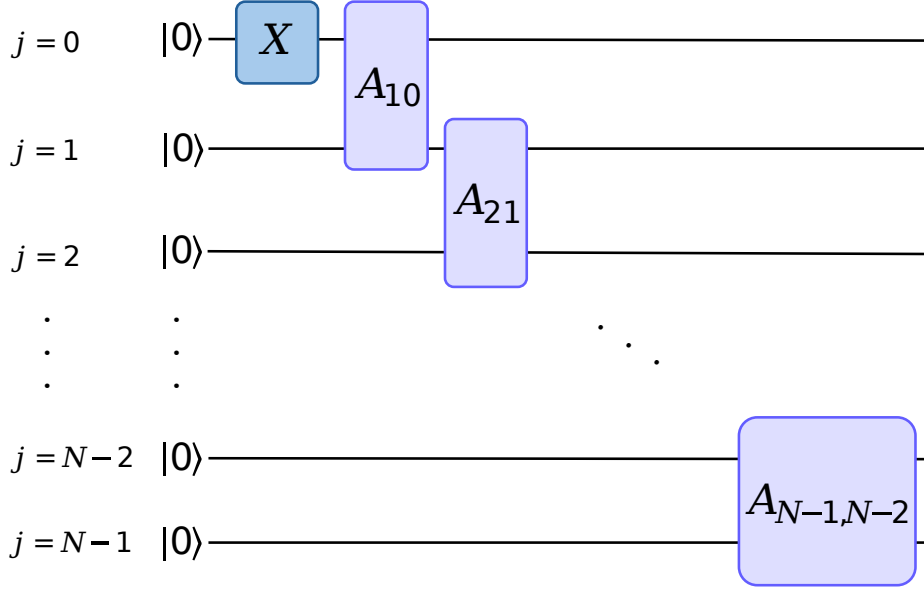

**Fig. 2:** Quantum circuit representation of an ansatz state (11).

superposition of the states of Hamming weight 1, i.e., the computational basis states that contain exactly one '1' and the remaining qubits in the state '0'. For an  $N$ -qubit system, the basis states are

$$|10\dots 0\rangle, |010\dots 0\rangle, \dots, |0\dots 01\rangle. \quad (12)$$

We may express our variational trial state as

$$|\psi\rangle = \sum_{j=0}^{N-1} a_j |e_j\rangle, \text{ where } a_j = |a_j| e^{i\phi_j}, \quad (13)$$

where  $|e_j\rangle$  are the basis states with '1' in the  $j$ -th position and '0' elsewhere. The coefficients  $a_j$  are, in general, complex numbers, expressed here in the complex exponential form with magnitude  $|a_j|$ , and phase  $\phi_j$ .

Let us calculate the expectation values of the operators  $\hat{Z}_j$ ,  $\hat{X}_j \hat{X}_l$ ,  $\hat{Y}_j \hat{Y}_l$ ,  $\hat{X}_j \hat{Y}_l$ , and  $\hat{Y}_j \hat{X}_l$ , respectively. First, the expectation value of  $\hat{Z}_j$  is

$$\begin{aligned} \langle \hat{Z}_j \rangle &= \sum_k a_k^* \langle e_k | \hat{Z}_j \sum_{k'} a_{k'} | e_{k'} \rangle = \sum_k a_k^* \langle e_k | \left( -a_j | e_j \rangle + \sum_{k' \neq j} a_{k'} | e_{k'} \rangle \right) \\ &= -a_j \sum_k a_k^* \delta_{kj} + \sum_{k, k' \neq j} a_k^* a_{k'} \delta_{kk'} = -|a_j|^2 + \sum_{k' \neq j} |a_{k'}|^2, \end{aligned} \quad (14)$$

where we used the fact that  $\hat{Z}_j$  acts non-trivially only when  $k' = j$ . Using the normalization condition  $\sum_{k=0}^{N-1} |a_k|^2 = 1$ , the resulting expression can be rewritten in a more convenient form

$$\langle \hat{Z}_j \rangle = -|a_j|^2 + \sum_{k' \neq j} |a_{k'}|^2 = 1 - 2|a_j|^2. \quad (15)$$

The second term is  $\langle \hat{X}_j \hat{X}_l \rangle = \langle \psi | \hat{X}_j \hat{X}_l | \psi \rangle$ . Consider the action of the operator  $\hat{X}_j \hat{X}_l$  on the state  $|\psi\rangle$ . If  $j, l \neq k$ , this will create the state with the Hamming weight 3, which does not belong to the subspace of Hilbert space where the solution is. The application of the bra vector from the left will result in zero overlap with such states due to the orthogonality. The only nontrivial results are when  $j = k, l \neq k$ , or  $l = k, j \neq k$ . Because of these relations, only two basis states are non-zero from the entire superposition

$$\sum_k a_k \hat{X}_j \hat{X}_l | e_k \rangle = a_j | e_l \rangle + a_l | e_j \rangle. \quad (16)$$

Here, we use the fact that  $\hat{X} | 1 \rangle = | 0 \rangle$ , and  $\hat{X} | 0 \rangle = | 1 \rangle$ . The application of the bra vector  $\langle \psi |$  gives us the expectation value.

$$\langle \hat{X}_j \hat{X}_l \rangle = \sum_k a_k^* \langle e_k | (a_j | e_l \rangle + a_l | e_j \rangle) = a_l^* a_j + a_j^* a_l = 2|a_j||a_l| \cos \varphi_{jl}, \quad (17)$$

where we defined the relative phases as  $\varphi_{jl} = \phi_l - \phi_j$ . Consider now the second expectation value  $\langle \hat{Y}_j \hat{Y}_l \rangle = \langle \psi | \hat{Y}_j \hat{Y}_l | \psi \rangle$ . Again, the action of the operator  $\hat{Y}_j \hat{Y}_l$  on the state  $|\psi\rangle$  gives nontrivial results only when  $j = k, l \neq k$ , or  $l = k, j$  and because  $\hat{Y}|0\rangle = i|1\rangle$ , and  $\hat{Y}|1\rangle = -i|0\rangle$ , we get

$$\sum_k a_k \hat{Y}_j \hat{Y}_l |e_k\rangle = -i^2 (a_j |e_l\rangle + a_l |e_j\rangle) = a_j |e_l\rangle + a_l |e_j\rangle, \quad (18)$$

and the resulting expectation value is

$$\langle \hat{Y}_j \hat{Y}_l \rangle = \sum_k a_k^* \langle e_k | (a_j |e_l\rangle + a_l |e_j\rangle) = a_l^* a_j + a_j^* a_l = 2|a_j||a_l| \cos \varphi_{jl}, \quad (19)$$

demonstrating that  $\langle \hat{X}_j \hat{X}_l \rangle = \langle \hat{Y}_j \hat{Y}_l \rangle$ . Similarly, we calculate the expectation values of the mixed operators  $\langle \hat{X}_j \hat{Y}_l \rangle$ ,  $\langle \hat{Y}_j \hat{X}_l \rangle$ . First, we obtain

$$\begin{aligned} \langle \hat{X}_j \hat{Y}_l \rangle &= \sum_{k'} a_{k'}^* \langle e_{k'} | \left( \sum_k a_k \hat{X}_j \hat{Y}_l |e_k\rangle \right) = \sum_{k'} a_{k'}^* \langle e_{k'} | (ia_j |e_l\rangle - ia_l |e_j\rangle) \\ &= i \sum_{k'} (a_{k'}^* a_j \delta_{k'l} - a_{k'}^* a_l \delta_{k'j}) = i (a_l^* a_j - a_j^* a_l) = 2|a_j||a_l| \sin \varphi_{jl}. \end{aligned} \quad (20)$$

And for the second operator, we have

$$\begin{aligned} \langle \hat{Y}_j \hat{X}_l \rangle &= \sum_{k'} a_{k'}^* \langle e_{k'} | \left( \sum_k a_k \hat{Y}_j \hat{X}_l |e_k\rangle \right) = \sum_{k'} a_{k'}^* \langle e_{k'} | (-ia_j |e_l\rangle + ia_l |e_j\rangle) \\ &= -i \sum_{k'} (a_{k'}^* a_j \delta_{k'l} - a_{k'}^* a_l \delta_{k'j}) = -i (a_l^* a_j - a_j^* a_l) = -2|a_j||a_l| \sin \varphi_{jl}, \end{aligned} \quad (21)$$

which shows that  $\langle \hat{X}_j \hat{Y}_l \rangle = -\langle \hat{Y}_j \hat{X}_l \rangle$ . Using the results (15), (17), (19), (20), and (21), the cost function of the qubit Hamiltonian, see Eq. (5) can be expressed as

$$E(\mathbf{k}, \boldsymbol{\theta}) = \sum_{j=0}^{N-1} \varepsilon_j |a_j|^2 + \sum_{j=0}^{N-2} \sum_{l>j} \text{Re}\{C_{jl} \mathcal{H}_{jl}(\mathbf{k})\}, \quad (22)$$

where the Pauli correlators  $C_{jl}$  encodes the the expectation value of the hopping terms in the variational state and are given by

$$C_{jl} = \langle \hat{X}_j \hat{X}_l \rangle + i \langle \hat{X}_j \hat{Y}_l \rangle = 2|a_j||a_l| e^{i\varphi_{jl}}. \quad (23)$$

To estimate the cost function (22), one needs to obtain the probabilities  $|a_j|^2$ , and the Pauli correlators  $C_{jl}$ , Eq. (23), that depend both on the variational parameters  $\boldsymbol{\theta}$ . These can be estimated with only three rounds of measurement settings, as discussed in the main text.

## Supplementary References

- [1] Preskill, J. Quantum computing in the nisc era and beyond. *Quantum* **2**, 79 (2018).
- [2] Higgott, O., Wang, D. & Brierley, S. Variational quantum computation of excited states. *Quantum* **3**, 156 (2019).
- [3] Peruzzo, A. *et al.* A variational eigenvalue solver on a photonic quantum processor. *Nat. Commun.* **5**, 4213 (2014).
- [4] Havlíček, V. *et al.* Supervised learning with quantum-enhanced feature spaces. *Nature* **567**, 209–212 (2019).
- [5] Gard, B. T. *et al.* Efficient symmetry-preserving state preparation circuits for the variational quantum eigensolver algorithm. *npj Quantum Inf.* **6**, 10 (2020).
- [6] Sherbert, K., Cerasoli, F. & Buongiorno Nardelli, M. A systematic variational approach to band theory in a quantum computer. *RSC Adv.* **11**, 39438–39449 (2021).
- [7] Sherbert, K., Jayaraj, A. & Buongiorno Nardelli, M. Quantum algorithm for electronic band structures with local tight-binding orbitals. *Sci. Rep.* **12**, 9867 (2022).
- [8] Ďuriška, M., Miháliková, I. & Friák, M. Quantum computing of the electronic structure of crystals by the variational quantum deflation algorithm. *Phys. Scr.* **100**, 045105 (2025).
- [9] Miháliková, I., Krejčí, M. & Friák, M. The impact of quantum circuit architecture and hyperparameters on variational quantum algorithms exemplified in the electronic. *Sci. Rep.* **15**, 15746 (2025).
